# Supplementary material for: Formal Development of Safe Automated Driving using Differential Dynamic Logic
Source: arXiv:2204.06873 source file (2022-04-14)
Supplement: Supplementary file 1 [file 9_0_appendix.tex]

\begin{equation}
    \mone \triangleq v\Tau + \frac{\aMaxN\,\Tau^2}{2} + \frac{\left(v+\aMaxN\,\Tau\right)^2}{2\aMinS}
\end{equation}
\begin{equation}
    \mthree \triangleq v\Tau + \dfrac{a_n \Tau^2}{2} + \dfrac{\left(v+a_n \Tau\right)^2}{2\aMinS}.
\end{equation}
\begin{equation}
    \mfive \triangleq v\Tau+\dfrac{a_n\Tau^2}{2} + \dfrac{\left(v + a_n\Tau\right)^2}{2\aMinN}.
\end{equation}
In Model~\ref{alg:sm5}, threat metric in acceleration domain but can be reformulated in distance domain...
\begin{align}
    \aReq \ge \ath \\
    -\dfrac{\left(v + a_n\Tau\right)^2}{2\left(x_c-x-v\Tau-\dfrac{a_n\Tau^2}{2}\right)}  \ge -\aMinN \\
     \left(v + a_n\Tau\right)^2 \le 2\left(x_c-x-v\Tau-\dfrac{a_n\Tau^2}{2}\right)\aMinN \\
     \dfrac{\left(v + a_n\Tau\right)^2}{2\aMinN} \le x_c-x-v\Tau-\dfrac{a_n\Tau^2}{2} \\
     x_c - x \ge v\Tau+\dfrac{a_n\Tau^2}{2} + \dfrac{\left(v + a_n\Tau\right)^2}{2\aMinN}
\end{align}
The following formula is proved in \keyx and shows that \mthree is indeed the better model. 
\begin{align*}
    \forall\begin{pmatrix} \aMinS \\ \aMinN \\ \aMaxN \\ \Tau \\ \vel \\ a_n \end{pmatrix}
    \Biggl( \left(\begin{bmatrix} 0 \\ 0 \\ 0 \\ \aMinN          \end{bmatrix} <
    \begin{bmatrix} \aMinN \\ \aMaxN \\ \Tau \\ \aMinS \end{bmatrix} \land 
    0 \le v \land -\aMinN \le a_n \le \aMaxN
    \right) \to \\
    (\mone \ge \mthree \land \mfive \ge \mthree)\Biggr)
\end{align*}
However, the following formula to show the relation between \mone and \mfive requires an extra condition. 
\begin{align*}
    \forall\begin{pmatrix} \aMinS \\ \aMinN \\ \aMaxN \\ \Tau \\ \vel \\ a_n \end{pmatrix}
    \Biggl( \left(\begin{bmatrix} 0 \\ 0 \\ 0 \\ \aMinN          \end{bmatrix} <
    \begin{bmatrix} \aMinN \\ \aMaxN \\ \Tau \\ \aMinS \end{bmatrix} \land 
     \begin{bmatrix} 0 \\ \dfrac{\left(v + a_n\Tau\right)^2}{\left(v + \aMaxN\Tau\right)^2} \end{bmatrix} \le
    \begin{bmatrix} 0 \\ \dfrac{\aMinS}{\aMinN} \end{bmatrix} \land \right. \\ 
    \left.\vphantom{\begin{bmatrix} 0 \\ 0 \\ 0 \\ \aMinN          \end{bmatrix}} -\aMinN \le a_n \le \aMaxN \right) \to (\mone \ge \mthree \land \mone \ge \mfive)\Biggr)
\end{align*}
From the above formulas, we can then conclude $(\mone \ge \mfive \land \mfive \ge \mthree)$ when the respective assumptions hold.
